# Supplementary material for: Graph matching between bipartite and unipartite networks: to collapse, or not to collapse, that is the question
Source: arXiv:2002.01648 source file (2021-04-12)
Supplement: Supplementary file 1 [file appendix_other.tex]

The graph matching solution is correct if
$${\ell}_m(\hat{\Theta}_{P^\ast}) < {\ell}_m(\hat{\Theta}_{P})\quad\quad\quad\text{for all }P\in\mathcal{P}\setminus\{P^\ast\}.$$
Therefore, we need to analyze/impose conditions on the following two main quantities:

\begin{enumerate}
    \item The global minimum of the expected likelihood needs to be sufficiently away from the minimums for each $P$, that is
    $$\ell^\ast(\widetilde{\Theta}_{P})- \ell^\ast({\Theta}^\ast) >  C_P>0,$$
    for some $C_P$ sufficiently large. In particular, suppose that the function $\ell^\ast$ satisfies strong convexity, i.e., 
    $$\ell^\ast(\Theta_1) - \ell^\ast(\Theta_2) \geq \left\langle\nabla\ell^\ast(\Theta_2), \Theta_1 - \theta_2)\right\rangle + \frac{\mu}{2}\|\Theta_1 - \Theta_2\|^2_F.$$
    Hence, it is enough that
    $$\ell^\ast(\widetilde{\Theta}_{P})- \ell^\ast({\Theta}^\ast) \geq \frac{\mu}{2}\|\widetilde{\Theta}_P - \Theta^\ast\|^2_F > C_P. $$ 
    This condition is still hard to check since it depends in several unknown parameters, so alternatively, we consider the following:
    \begin{align*}
        \|\widetilde{\Theta}_P - \Theta^\ast\|^2_F   & \geq  \argmin_{\Theta\in\mathcal{M}(P)}\|\Theta - \Theta^\ast\|^2_F\\
        & = \argmin_{\Theta\in\mathcal{M}(P)}\left\{\sum_{i=1}^n\sum_{j=1}^n (\Theta_{ij} - \Theta^\ast_{ij})^2 \right\}\\
        & \geq \sum_{(i,j)\in\mathcal{U}_3}(\Theta^\ast_{ij})^2 \\ 
        & \geq |\mathcal{U}_3| \min_{(i,j)\in\mathcal{U}_3}|\Theta^\ast_{ij}|^2
    \end{align*}
    $\mathcal{U}=[n]\times [n]$, $\mathcal{U} = \mathcal{U}_1 \cup \mathcal{U}_2 \cup \mathcal{U}_3$, where
    $$\mathcal{U}_1 = \{(i,j)\in\mathcal{U}: A_{ij} = (PAP^T)_{ij}\},$$
    $$\mathcal{U}_2 = \{(i,j)\in\mathcal{U}: A_{ij} = 0, (PAP^T)_{ij}=1\}.$$
    $$\mathcal{U}_3 = \{(i,j)\in\mathcal{U}: A_{ij} = 1, (PAP^T)_{ij}=0\},$$
    
    $|\mathcal{U}_3|\overset{?}{=}\frac{1}{2}\|A-PAP^T\|_F^2$
    
    \item The empirical and expected likelihoods need to be sufficiently close, i.e., 
    $$|\ell_m(\widehat\Theta)- \ell^\ast(\Theta^\ast)|< C_2$$
    $$|\ell_m(\widehat\Theta_P)- \ell^\ast(\widetilde\Theta_P)| < C_{3,P}.$$
    The above inequalities imply that
    \begin{align*}
        \ell_m(\widehat\Theta) & \leq |\ell_m(\widehat\Theta) - \ell^\ast(\Theta^\ast)| + \ell^\ast(\Theta^\ast)\\
        & \leq C_2 - C_P + \ell^\ast(\widetilde\Theta_P)\\
        & = C_2 - C_P + \ell^\ast(\widetilde\Theta_P) - \ell_m(\widehat\Theta_P) + \ell_m(\widehat\Theta_P)\\
        &\leq C_2 - C_P + |\ell^\ast(\widetilde\Theta_P) - \ell_m(\widehat\Theta_P) |+ \ell_m(\widehat\Theta_P)\\
        & \leq C_2 - C_P + C_{3,P} + \ell_m(\widehat\Theta_P).
    \end{align*}
    Therefore, a sufficient condition for $\ell_m(\widehat\Theta) < \ell_m(\widehat\Theta_P) $ (i.e., correct recovery of the unshuffling permutation) is that
    $C_2 + C_{3,P} < C_P,$
    or equivalently
    \begin{equation}
    |\ell_m(\widehat\Theta)- \ell^\ast(\Theta^\ast)|  + |\ell_m(\widehat\Theta_P)- \ell^\ast(\widetilde\Theta_P)| <   \frac{\mu}{2}\|\widetilde{\Theta}_P - \Theta^\ast\|^2_F. \label{eq:sufficient-condition}    
    \end{equation}
\end{enumerate}

Now, to bound the difference between the empirical and expected likelihoods, observe that
\begin{align}
    |\ell_m(\widehat{\Theta}_P) - \ell^\ast(\widetilde\Theta_P)|  & \leq |\ell_m(\widehat{\Theta}_P)-\ell_m(\widetilde\Theta_P)| +|\ell_m(\widetilde\Theta_P)- \ell^\ast(\widetilde\Theta_P)|. \label{eq:empirical-likelihood-error}
\end{align}

Convexity of the loss function implies that the first term in Equation~\eqref{eq:empirical-likelihood-error} is bounded from above by
\begin{align*}
    |\ell_m(\widehat{\Theta}_P)-\ell_m(\widetilde\Theta_P)| & = \ell_m(\widetilde\Theta_P) -\ell_m(\widehat{\Theta}_P)\\
    & \leq \left\langle \nabla \ell_m(\widetilde\Theta_P), \widetilde\Theta_P  - \widehat{\Theta}_P\right\rangle\\
    & \leq \|A\cdot \nabla \ell_m(\widetilde\Theta_P)\|_F\|\widetilde\Theta_P  - \widehat{\Theta}\|_F\\
    & = \|A\cdot \widehat{\Sigma}-A\cdot \Sigma^\ast\|_F\|\widetilde\Theta_P  - \widehat{\Theta}_P\|_F.
\end{align*}
Write $\ell_{m,P}$ as
\begin{equation*}
    \ell_{m,P}(\theta) = \frac{1}{m}\sum_{k=1}^m\left(\sum_{(i,j)\in \mathcal{U}(P)} \theta_{[i,j]}B_{ik}B_{ijk} - 2\sum_{i=1}^n\Theta_{ii}C(B_{ik}\right),
\end{equation*}
and $\ell_P(\theta) = \mathbb{E}[\ell_{m,P}(\theta)]$. 
Assume the following conditions
\begin{itemize}
    \item Lipschitz continuity of $\ell_P$ (yes, because of convexity)
    \item $\nabla^2\ell_{P}(\widetilde\theta_P)$ is an invertible matrix for all $\widetilde\theta_P$
    \item Set $\Phi_P = (\nabla^2\ell_{P}(\widetilde\theta_P))^{-1}\nabla\ell_{P}(\widetilde\theta_P)(\nabla^2\ell_{P}(\widetilde\theta_P)])^{-1}$. Assume $\Phi_P$ is invertible, and that $\|\Phi_P\| = O(1)$.
    \item $\widehat\Theta_P\overset{P}{\rightarrow}\widetilde\Theta_P$ (true because of first part of the theorem).
\end{itemize}
By Theorem 5.21 of \cite{van2000asymptotic} (asymptotic normality of M-estimators), we have
\begin{equation*}
    \sqrt{m}(\widehat{\theta}_P - \widetilde\theta_P ) \overset{d}{\rightarrow} N(0, \Phi).
\end{equation*}
Therefore,
\begin{align*}
\|\widehat{\Theta}_P - \widetilde\Theta_P \|_F & = \|\widehat{\theta}_P - \widetilde\theta_P \|\\
& = \|\Phi^{1/2}_P\|\|\Phi^{-1/2}_P(\widehat{\theta}_P - \widetilde\theta_P)\|\\
& = O_P\left(\frac{\sqrt{dn}}{\sqrt{m}}\right).
\end{align*}

On the other hand, by \cite{Levina2012}
\begin{align*}
    \|A\cdot \widehat{\Sigma}-A\cdot \Sigma^\ast\|_F & \leq \sqrt{n}\|A\cdot \widehat{\Sigma}-A\cdot \Sigma^\ast\|\\
    & = O_P\left(\|\Sigma^\ast\|\log^3 (n) \left(\frac{\sqrt{nd}}{\sqrt{m}} + \frac{d\sqrt{n}}{m} \right) \right)
\end{align*}

Now, to control the second term in Equation~\eqref{eq:empirical-likelihood-error}, substituting the log-likelihood function~\eqref{eq:GLM-full} (when $\beta=0$)
\begin{align*}
    |\ell_m(\widetilde\Theta_P)- \ell^\ast(\widetilde\Theta_P)| & = \left|\frac{1}{m}\sum_{k=1}^m\left\{\sum_{i\neq j}  (\widetilde\Theta_P)_{ij}(B_{ik}B_{jk} - \e[B_{ik}B_{jk}]) + \sum_{i=1}^n\Theta_{ii}(C(B_{ik})-\e[C(B_{ik})])\right\}  \right|\\
    & =  |\left\langle\nabla\ell_m(\widetilde\Theta_P) - \nabla \ell^\ast(\widetilde\Theta_P), \widetilde\Theta_P\right\rangle|.\\
    & \leq \|A\cdot \nabla\ell_m(\widetilde\Theta_P) - A\cdot \nabla \ell^\ast(\widetilde\Theta_P)\|_F\|\widetilde\Theta_P\|_F
\end{align*}
For a Gaussian distribution, observe that
\begin{align*}
    \|A\cdot\nabla\ell_m(\widetilde\Theta_P) - A\cdot\nabla \ell^\ast(\widetilde\Theta_P)\|_F & = \|A\cdot\widehat\Sigma - A\cdot\Sigma^\ast\|_F
\end{align*}
Therefore,
$$ |\ell_m(\Theta^\ast)- \ell^\ast(\Theta^\ast)|\leq \|A\cdot\widehat{\Sigma}-A\cdot\Sigma^\ast\|_F\|\Theta^\ast\|_F.$$
Combining these bounds, Eq.~\eqref{eq:empirical-likelihood-error} becomes
\begin{equation*}
    |\ell_m(\widehat{\Theta}) - \ell^\ast(\Theta^\ast)| \leq \|A\cdot\widehat{\Sigma}-A\cdot\Sigma^\ast\|_F(\|\Theta^\ast\|_F + \|\Theta^\ast  - \widehat{\Theta}\|_F) .
\end{equation*}

Let's apply the previous analysis to a gaussian distribution. First notice that
$$\ell_m(\Theta) = \text{Tr}(\widehat{\Sigma}\Theta) - \log\text{det}(\Theta)$$
$$\nabla\ell_m(\Theta) = \widehat{\Sigma} - \Theta^{-1}$$
$$\nabla\ell_m(\Theta)^\ast = \widehat{\Sigma} - \Sigma^\ast$$

Therefore, combining everything together into equation \eqref{eq:sufficient-condition},

\begin{align*}
    |\ell_m(\widehat\Theta)- \ell^\ast(\Theta^\ast)|  + |\ell_m(\widehat\Theta_P)- \ell^\ast(\widetilde\Theta_P)| \leq & \|A\cdot\widehat{\Sigma}-A\cdot\Sigma^\ast\|_F(\|\Theta^\ast\|_F + \|\widetilde\Theta_P\|_F \\
    & +\|\Theta^\ast  - \widehat{\Theta}\|_F + +\|\widetilde\Theta_P  - \widehat{\Theta}_P\|_F)\\
    =& O_P\left(\|\Sigma^\ast\|\log^3 (n) \left(\frac{\sqrt{nd}}{\sqrt{m}} + \frac{d\sqrt{n}}{m} \right)\left(\sqrt{\frac{nd}{m}} + \sqrt{nd} \right) \right) \\
    & \frac{\mu}{2}\|\widetilde{\Theta}_P - \Theta^\ast\|^2_F.
\end{align*}
This implies that the MLE recovers the shuffling permutation with probability tending to one as long as
\begin{equation*}
    \|\Sigma^\ast\|\log^3 (n) \left(\frac{{nd}}{\sqrt{m}} + \frac{d^{3/2}{n}}{m} \right)\leq \mu \min_{P\in\Pi_n}\|A - PAP^T\|_F^2,
\end{equation*}
provided that $|\Theta^\ast_{ij}|\asymp 1$ for all $A_{ij}=1$ and $|(\widetilde \Theta_P)_{ij}|\asymp 1$ for all $(PAP^T)_{ij}=1$. In particular, observe that the right hand side is upper bounded by $d$, so the proof requires a sample size of at least $m>n^2$.
